# Supplementary material for: A Systematic Modeling Framework for Dynamic Simulation of Fixed-Bed Reactors
Source: arXiv:2604.22468 source file (2026-04-24)
Supplement: Supplementary file 1 [file advection_appendixversion.tex]

\section{Pressure-drop relations}\label{app:pressuredrop}
Different semi-empirical relations are relevant for different types of reactor volumes and for different flow regimes. Here, we briefly summarize some of the most prevalent models for steady flow in tubular and fixed-bed reactor volumes.

For tubular volumes, we relate the velocity $v$ to the pressure drop $\partial_zP$ via the semi-empirical Darcy-Weisbach equation
\begin{align}\label{eq:darcyweisbach}
    -\partial_zP=\frac{f_{DW}\rho}{2d}v|v|,
\end{align}
where $f_{DW}$~[-] denotes the Darcy-Weisbach friction factor. For fully developed flow, which is common in industrial reactors, the friction factor is written as a function of two dimensionless quantities
\begin{align}
    f_{DW}=f_{DW}(\text{Re},\eta),
\end{align}
the Reynolds number \text{Re}~[-] and the relative tube roughness $\eta$ [-]. The Reynolds number is defined by
\begin{align}
    \text{Re}=\frac{\rho d |v|}{\mu},
\end{align}
where the relative tube roughness is defined by $\eta=d/h$, where $h$ [m] denotes the tube roughness height. For laminar flow ($\text{Re}<2\,000$), the friction factor depends solely on the Reynolds number. Conversely, for highly turbulent flow ($\text{Re}>2\,000\,000$), the friction factor is said to depend only on the relative tube roughness. In transitional and turbulent flow regimes, which are common in industrial reactors, we consider both and present the Colebrook-White equation. It provides the implicit logarithmic law
\begin{align}\label{eq:colebrookwhite}
    \frac{1}{\sqrt{f_{DW}}}=-2\log_{10}\left(\frac{2.51}{\text{Re}\sqrt{f_{DW}}}+\frac{\eta}{3.71}\right).
\end{align}
Because of its implicit nature, there has been extensive study of explicit approximations of \eqref{eq:colebrookwhite}, including Moody's work, which laid the foundation for the famous Moody diagram. We refer to the review of explicit power-law and logarithmic-law approximations found in \cite{brkic2011review}.

For heterogeneous volumes, we study the superficial velocity $v_s=\varepsilon v$ [m$/$s] which is the product of the (interstitial) velocity $v$ [m$/$s] and the void fraction $\varepsilon$ [-]. The void fraction for a heterogeneous subvolume $\sigma$ is defined as $\varepsilon=\varphi_{\sigma,\text{fluid}}$, as in \eqref{eq:fractions}. We relate the superficial velocity to the pressure drop via the general Ergun equation
\begin{align}\label{eq:generalergun}
    -\partial_zP=\frac{f_{E}\mu(1-\varepsilon)^2}{d_p^2\varepsilon^3}v_s,
\end{align}
where $f_{E}$ [-] denotes the Ergun friction factor and $d_p$ [m] denotes the solid-phase particle diameter. The Ergun friction factor is written as a function of the modified Reynolds number $\widetilde{\text{Re}}$ [-] which is defined as
\begin{align}
    \widetilde{\text{Re}}=\frac{\rho d_p|v_s|}{\mu(1-\varepsilon)}.
\end{align}
In this way, the classical Ergun equation is simply summarized by a power law for the friction factor
\begin{align}
    f_{E}&=150+1.75\widetilde{\text{Re}},
\end{align}
which inserted into \eqref{eq:generalergun} gives a quadratic formula 
\begin{align}\label{eq:classicalergun}
    -\partial_zP=\frac{150\mu(1-\varepsilon)^2}{d_p^2\varepsilon^3}v_s+\frac{1.75\rho(1-\varepsilon)}{d_p\varepsilon^3}v_s|v_s|.
\end{align}
The Ergun equation is reasonable for laminar and early transitional flow ($\widetilde{\text{Re}}<500$). However, despite its popularity, the Ergun equation is not well suited for late transitional or turbulent flow ($\widetilde{\text{Re}}\gg500$) \citep{hicks1970pressure}. For more generally applicable friction factors, we refer to the review in \cite{erdim2015revisit}.
